# Supplementary material for: QUAR-VLA: Vision-Language-Action Model for Quadruped Robots
Source: arXiv:2312.14457 source file (2025-02-04)
Supplement: Supplementary file 1 [file table_s_arch.tex]

\begin{table*}[t]
\scriptsize
% 行距
\centering
\caption{Details of Architecture. }
\setlength{\tabcolsep}{2mm}{
\begin{tabular}{@{}cccc@{}}
\toprule
layer name       & input size                              & hyperparameters                                                                                                                                                                                                                                              & output size     \\ \midrule
DCT              & (75/45/45)×T                            &                                                                                                                                                                                                                                                              & (75/45/45)×$H_c$ \\\midrule
Replicate        & (75/45/45)×$H_c$                         &                                                                                                                                                                                                                                                              & (75/48/48)×$H_c$ \\\midrule
GCN\_1           & (75/48/48)×$H_c$                         & \begin{tabular}[c]{@{}c@{}}Graph 75×75/48×48/48×48, H;\\ BN,Tanh,Dropout\end{tabular}                                                                                                                                                                     & (75/48/48)×H    \\\midrule
12 GCN\_Blocks   & (75/48/48)×H                            & \begin{tabular}[c]{@{}c@{}}Graph 75×75/48×48/48×48, H;\\ BN, Tanh, Dropout;\\ Graph 75×75/48×48/48×48, H;\\ BN, Tanh, Dropout;\\ ...(×12)\\ Graph 75×75/48×48/48×48, H;\\ BN, Tanh, Dropout;\\ Graph 75×75/48×48/48×48, H;\\ BN, Tanh, Dropout;\end{tabular} & (75/48/48)×H    \\\midrule
DN\_ml           & 75×H; 48×H                              &                                                                                                                                                                                                                                                              & 75×H; 48×H      \\\midrule
DN\_mr           & 75×H; 48×H                              &                                                                                                                                                                                                                                                              & 75×H; 48×H      \\\midrule
DN\_rl           & 48×H; 48×H                              &                                                                                                                                                                                                                                                              & 48×H; 48×H      \\\midrule
5 SI\_Blocks\_ml & 75×H; 48×H                              & \begin{tabular}[c]{@{}c@{}}Attention, Add\&LN;\\ Linear(H×4H), ReLU, Dropout, Linear(4H×H), Dropout\\ …(×5)\\ Attention, Add\&LN;\\ Linear(4H×H), ReLU, Dropout, Linear(4H×H)\end{tabular}                                                                & 75×H            \\\midrule
5 SI\_Blocks\_mr & 75×H; 48×H                              & \begin{tabular}[c]{@{}c@{}}Attention, Add\&LN;\\ Linear(H×4H), ReLU, Dropout, Linear(4H×H) , Dropout\\ …(×5)\\ Attention, Add\&LN;\\ Linear(4H×H), ReLU, Dropout, Linear(4H×H)\end{tabular}                                                                & 75×H            \\\midrule
5 SI\_Blocks\_lm & 48×H;75×H                               & \begin{tabular}[c]{@{}c@{}}Attention, Add\&LN;\\ Linear(H×4H), ReLU, Dropout, Linear(4H×H) , Dropout\\ …(×5)\\ Attention, Add\&LN;\\ Linear(4H×H), ReLU, Dropout, Linear(4H×H)\end{tabular}                                                                & 48×H            \\\midrule
5 SI\_Blocks\_lr & 48×H; 48×H                              & \begin{tabular}[c]{@{}c@{}}Attention, Add\&LN;\\ Linear(H×4H), ReLU, Dropout, Linear(4H×H) , Dropout\\ …(×5)\\ Attention, Add\&LN;\\ Linear(4H×H), ReLU, Dropout, Linear(4H×H)\end{tabular}                                                                & 48×H            \\\midrule
5 SI\_Blocks\_rm & 48×H;75×H                               & \begin{tabular}[c]{@{}c@{}}Attention, Add\&LN;\\ Linear(H×4H), ReLU, Dropout, Linear(4H×H) , Dropout\\ …(×5)\\ Attention, Add\&LN;\\ Linear(4H×H), ReLU, Dropout, Linear(4H×H)\end{tabular}                                                                & 48×H            \\\midrule
5 SI\_Blocks\_rl & 48×H; 48×H                              & \begin{tabular}[c]{@{}c@{}}Attention, Add\&LN;\\ Linear(H×4H), ReLU, Dropout, Linear(4H×H) , Dropout\\ …(×5)\\ Attention, Add\&LN;\\ Linear(4H×H), ReLU, Dropout, Linear(4H×H)\end{tabular}                                                                & 48×H            \\\midrule
Concat           & (75/48/48)×H;(75/48/48)×H;(75/48/48)×H; &                                                                                                                                                                                                                                                              & (75/48/48)×3H   \\\midrule
PI\_Block\_rm    & 75×3H;48×3H                             & Linear(H×H×1), Weighted Sum                                                                                                                                                                                                                                  & 75×3H;45×3H     \\\midrule
PI\_Block\_lm    & 75×3H;48×3H                             & Linear(H×H×1), Weighted Sum                                                                                                                                                                                                                                  & 75×3H;45×3H     \\ \midrule
MLP              & (75/45/45)×3H                           & Linear(3H×$H_c$)                                                                                                                                                                                                                                              & (75/45/45)×$H_c$ \\\midrule
IDCT             & (75/45/45)×$H_c$                         &                                                                                                                                                                                                                                                              & (75/45/45)×$\Delta T$\\ \bottomrule  
\end{tabular}
}
\label{Table:arch}
\end{table*}
