# Supplementary material for: QUAR-VLA: Vision-Language-Action Model for Quadruped Robots
Source: arXiv:2312.14457 source file (2025-02-04)
Supplement: Supplementary file 3 [file table_s_moreaction.tex]

%%%%%%%%%%%%%%%%%%%%%%%%%%%%%%%%%%%%%%%%%%%%%%%%%%%%%%%%%%%%%%%%%%%%%%%
\begin{table*}[t!]
\caption{\textbf{Detailed results on other action split} with the evaluation metrics MPJPE (in $mm$). (U) is the abbreviation of united training strategy. The best results are highlighted in bold.
}
\vspace{-.5em}
%行距
\label{tab:s_moreaction}
\centering
\scriptsize
\setlength{\tabcolsep}{0.64mm}{
\begin{tabular}{cc|cccc|cccc|cccc|cccc|cccc|cccc}
\hline
\multicolumn{2}{c|}{Time (sec)} 
& 0.2 & 0.4 & 0.8 & 1.0 
& 0.2 & 0.4 & 0.8 & 1.0 
& 0.2 & 0.4 & 0.8 & 1.0 
& 0.2 & 0.4 & 0.8 & 1.0 
& 0.2 & 0.4 & 0.8 & 1.0 
& 0.2 & 0.4 & 0.8 & 1.0 
\\
\hline
\multicolumn{2}{c|}{Action} 
& \multicolumn{4}{c|}{ fly } 
& \multicolumn{4}{c|}{ see } 
& \multicolumn{4}{c|}{ peel } 
& \multicolumn{4}{c|}{ browse } 
& \multicolumn{4}{c|}{ takepicture } 
& \multicolumn{4}{c}{ inspect }  \\
{} & {LTD (U)~\cite{mao2019learning}}
 &29.1 &78.4 &170.0 &\textbf{181.7}
   &14.8 &43.0 &119.5 &153.6
   &27.3 &62.6 &111.1 &112.0
   &9.9 &23.2 &90.6 &133.4
   &\textbf{11.2} &\textbf{28.7} &115.0 &181.4
   &23.4 &59.2 &110.5 &120.6
\\
% {} & {DMGNN (U)~\cite{li2020dynamic}}
 
% \\
% {\cellcolor{white}} &{\cellcolor{white}PGBIG (U)~\cite{ma2022progressively}} 

% \\
{\cellcolor{white}} & {\cellcolor{white}SPGSN (U)~\cite{li2022skeleton}} 
&38.3 &88.6 &176.4 &211.2
   &20.3 &54.1 &124.7 &\textbf{140.7}
   &27.3 &\textbf{55.6} &\textbf{102.7} &\textbf{107.8}
   &11.7 &29.1 &54.0 &65.6
   &14.6 &33.3 &\textbf{108.3} &\textbf{165.2}
   &23.5 &56.9 &107.6 &121.7
\\
\multirow{-4}{*}{\rotatebox[origin=c]{90}{\cellcolor{white}\textbf{Whole body}}}
{\cellcolor{white}} &{\cellcolor{white} \textbf{EAI} (Ours)}
   &\textbf{26.1} &\textbf{70.7} &\textbf{160.0} &{188.1}
   &\textbf{14.2} &\textbf{42.5} &\textbf{114.3} &{143.9}
   &\textbf{24.8} &{59.3} &{113.4} &{118.6}
   &\textbf{7.3} &\textbf{18.8} &\textbf{38.3} &\textbf{49.1}
   &{11.8} &{33.4} &{112.1} &{165.5}
   &\textbf{21.2} &\textbf{55.3} &\textbf{106.8} &\textbf{115.7}
\\
\hline
\hline

%%%%%%%%%%%%. main body %%%%%%%%%%%%%%%%%%%%
\multicolumn{2}{c|}{Action} 
& \multicolumn{4}{c|}{ pour } 
& \multicolumn{4}{c|}{ use } 
& \multicolumn{4}{c|}{ wear } 
& \multicolumn{4}{c|}{ play } 
& \multicolumn{4}{c|}{ cook } 
& \multicolumn{4}{c}{ shake }  \\
{\cellcolor{white}} & {\cellcolor{white}LTD (U)~\cite{mao2019learning}}
&\textbf{23.1} &54.9 &83.3 &92.4
   &22.4 &57.5 &155.6 &185.9
   &\textbf{11.8} &\textbf{31.1} &87.9 &112.3
   &14.7 &39.3 &73.3 &92.2
   &25.7 &56.7 &86.3 &110.4
   &21.1 &\textbf{29.3} &\textbf{44.9} &52.0
\\
% {\cellcolor{white}} & {\cellcolor{white}DMGNN (U)~\cite{li2020dynamic}} 
  
% \\
% {\cellcolor{white}} &{\cellcolor{white}PGBIG (U)~\cite{ma2022progressively}} 

% \\
{\cellcolor{white}} & {\cellcolor{white}SPGSN (U)~\cite{li2022skeleton}} 
&27.1 &60.1 &85.6 &94.4
   &23.8 &59.1 &169.5 &207.4
   &13.7 &36.8 &89.5 &112.2
   &17.2 &40.3 &74.8 &90.6
   &29.8 &61.7 &\textbf{75.1} &\textbf{91.7}
   &28.5 &42.9 &72.4 &78.4
\\
\multirow{-4}{*}{\rotatebox[origin=c]{90}{\cellcolor{white}\textbf{Whole body}}}
{\cellcolor{white}} &{\cellcolor{white} \textbf{EAI} (Ours)}
&{24.6} &\textbf{53.7} &\textbf{79.0} &\textbf{81.4}
   &\textbf{19.4} &\textbf{51.6} &\textbf{145.5} &\textbf{178.1}
   &{13.9} &{35.6} &\textbf{76.7} &\textbf{96.1}
   &\textbf{12.0} &\textbf{32.6} &\textbf{68.2} &\textbf{86.4}
   &\textbf{23.7} &\textbf{50.1} &{76.8} &{100.3}
   &\textbf{18.3} &{33.9} &{45.1} &\textbf{49.5}
\\
\hline
\hline

%%%%%%%%%%%%. left hand %%%%%%%%%%%%%%%%%%%%
\multicolumn{2}{c|}{Action} 
& \multicolumn{4}{c|}{ chop } 
& \multicolumn{4}{c|}{ screw } 
& \multicolumn{4}{c|}{ toast } 
& \multicolumn{4}{c|}{ call } 
& \multicolumn{4}{c|}{ stamp } 
& \multicolumn{4}{c}{ staple }  \\
{\cellcolor{white}} & {\cellcolor{white}LTD (U)~\cite{mao2019learning}}
&\textbf{16.5} &\textbf{36.1} &67.7 &82.9
   &14.9 &31.5 &149.7 &214.6
   &16.7 &41.5 &\textbf{78.8} &117.1
   &\textbf{12.3} &33.1 &\textbf{83.7} &\textbf{100.2}
   &\textbf{12.8} &\textbf{22.7} &66.0 &124.2
   &\textbf{14.2} &\textbf{24.5} &\textbf{60.2} &91.1
\\
% {\cellcolor{white}} & {\cellcolor{white}DMGNN (U)~\cite{li2020dynamic}} 
 
% \\
% {\cellcolor{white}} &{\cellcolor{white}PGBIG(U)~\cite{ma2022progressively}}

% \\
{\cellcolor{white}} & {\cellcolor{white}SPGSN (U)~\cite{li2022skeleton}} 
   &20.2 &38.2 &\textbf{62.1} &\textbf{77.7}
   &13.8 &\textbf{30.2} &141.8 &200.7
   &17.7 &\textbf{41.0} &79.6 &121.5
   &12.6 &\textbf{32.1} &86.3 &107.1
   &16.0 &25.6 &\textbf{59.7} &\textbf{101.3}
   &18.8 &32.7 &62.6 &\textbf{90.9}
\\
\multirow{-4}{*}{\rotatebox[origin=c]{90}{\cellcolor{white}\textbf{Whole body}}}
{\cellcolor{white}} &{\cellcolor{white} \textbf{EAI} (Ours)}
&{18.4} &{37.9} &{67.0} &{79.9}
   &\textbf{13.4} &{31.5} &\textbf{113.7} &\textbf{135.0}
   &\textbf{15.5} &{41.2} &{91.1} &\textbf{104.8}
   &{12.7} &{38.4} &{91.4} &{111.4}
   &{14.2} &{27.2} &{77.5} &{126.2}
   &{14.9} &{30.0} &{67.9} &{95.2}
\\
\hline
\hline

\hline
\end{tabular}}
\vspace{-.7em}
\end{table*}
%%%%%%%%%%%%%%%%%%%%%%%%%%%%%%%%%%%%%%%%%%%%%%%%%%%%%%%%%%%%%%%%%%%%%%%%
