# Supplementary material for: QUAR-VLA: Vision-Language-Action Model for Quadruped Robots
Source: arXiv:2312.14457 source file (2025-02-04)
Supplement: Supplementary file 4 [file table_s_suba.tex]

\begin{table*}[!ht]
\scriptsize
% 行距
\centering
\caption{145 sub-action types of S10. }
\vspace{-.5em}
\setlength{\tabcolsep}{4.5mm}{
\begin{tabular}{|lllll|}
\hline
\multicolumn{1}{|l|}{airplane-fly-1}       & \multicolumn{1}{l|}{cubemedium-lift-1}        & \multicolumn{1}{l|}{fryingpan-cook-2}      & \multicolumn{1}{l|}{phone-call-1}            & stapler-staple-2      \\ \hline
\multicolumn{1}{|l|}{airplane-lift-1}      & \multicolumn{1}{l|}{cubemedium-pass-1}        & \multicolumn{1}{l|}{gamecontroller-lift-1} & \multicolumn{1}{l|}{phone-lift-1}            & teapot-pass-1         \\ \hline
\multicolumn{1}{|l|}{airplane-pass-1}      & \multicolumn{1}{l|}{cubesmall-inspect-1}      & \multicolumn{1}{l|}{gamecontroller-pass-1} & \multicolumn{1}{l|}{phone-pass-1}            & teapot-pour-1         \\ \hline
\multicolumn{1}{|l|}{alarmclock-lift-1}    & \multicolumn{1}{l|}{cubesmall-lift-1}         & \multicolumn{1}{l|}{gamecontroller-play-1} & \multicolumn{1}{l|}{piggybank-pass-1}        & teapot-pour-2         \\ \hline
\multicolumn{1}{|l|}{alarmclock-pass-1}    & \multicolumn{1}{l|}{cubesmall-pass-1}         & \multicolumn{1}{l|}{hammer-lift-1}         & \multicolumn{1}{l|}{piggybank-use-1}         & toothpaste-lift-1     \\ \hline
\multicolumn{1}{|l|}{alarmclock-see-1}     & \multicolumn{1}{l|}{cup-drink-1}              & \multicolumn{1}{l|}{hammer-pass-1}         & \multicolumn{1}{l|}{pyramidlarge-pass-1}     & toothpaste-pass-1     \\ \hline
\multicolumn{1}{|l|}{apple-eat-1}          & \multicolumn{1}{l|}{cup-drink-2}              & \multicolumn{1}{l|}{hammer-use-1}          & \multicolumn{1}{l|}{pyramidmedium-inspect-1} & toothpaste-squeeze-1  \\ \hline
\multicolumn{1}{|l|}{apple-pass-1}         & \multicolumn{1}{l|}{cup-lift-1}               & \multicolumn{1}{l|}{hammer-use-2}          & \multicolumn{1}{l|}{pyramidmedium-lift-1}    & toothpaste-squeeze-2  \\ \hline
\multicolumn{1}{|l|}{banana-eat-1}         & \multicolumn{1}{l|}{cup-pass-1}               & \multicolumn{1}{l|}{hammer-use-3}          & \multicolumn{1}{l|}{pyramidmedium-pass-1}    & toruslarge-inspect-1  \\ \hline
\multicolumn{1}{|l|}{banana-lift-1}        & \multicolumn{1}{l|}{cup-pour-1}               & \multicolumn{1}{l|}{hand-inspect-1}        & \multicolumn{1}{l|}{pyramidsmall-inspect-1}  & toruslarge-lift-1     \\ \hline
\multicolumn{1}{|l|}{banana-pass-1}        & \multicolumn{1}{l|}{cylinderlarge-inspect-1}  & \multicolumn{1}{l|}{hand-lift-1}           & \multicolumn{1}{l|}{scissors-pass-1}         & toruslarge-pass-1     \\ \hline
\multicolumn{1}{|l|}{banana-peel-1}        & \multicolumn{1}{l|}{cylinderlarge-lift-1}     & \multicolumn{1}{l|}{hand-pass-1}           & \multicolumn{1}{l|}{scissors-use-1}          & torusmedium-inspect-1 \\ \hline
\multicolumn{1}{|l|}{banana-peel-2}        & \multicolumn{1}{l|}{cylinderlarge-pass-1}     & \multicolumn{1}{l|}{hand-shake-1}          & \multicolumn{1}{l|}{spherelarge-inspect-1}   & torusmedium-lift-1    \\ \hline
\multicolumn{1}{|l|}{binoculars-lift-1}    & \multicolumn{1}{l|}{cylindermedium-inspect-1} & \multicolumn{1}{l|}{headphones-lift-1}     & \multicolumn{1}{l|}{spherelarge-lift-1}      & torusmedium-pass-1    \\ \hline
\multicolumn{1}{|l|}{binoculars-pass-1}    & \multicolumn{1}{l|}{cylindermedium-pass-1}    & \multicolumn{1}{l|}{headphones-pass-1}     & \multicolumn{1}{l|}{spherelarge-pass-1}      & torussmall-inspect-1  \\ \hline
\multicolumn{1}{|l|}{binoculars-see-1}     & \multicolumn{1}{l|}{cylindersmall-inspect-1}  & \multicolumn{1}{l|}{headphones-use-1}      & \multicolumn{1}{l|}{spheremedium-inspect-1}  & torussmall-lift-1     \\ \hline
\multicolumn{1}{|l|}{bowl-drink-1}         & \multicolumn{1}{l|}{cylindersmall-pass-1}     & \multicolumn{1}{l|}{knife-chop-1}          & \multicolumn{1}{l|}{spheremedium-lift-1}     & torussmall-pass-1     \\ \hline
\multicolumn{1}{|l|}{bowl-drink-2}         & \multicolumn{1}{l|}{doorknob-lift-1}          & \multicolumn{1}{l|}{knife-pass-1}          & \multicolumn{1}{l|}{spheremedium-pass-1}     & train-lift-1          \\ \hline
\multicolumn{1}{|l|}{bowl-lift-1}          & \multicolumn{1}{l|}{doorknob-use-1}           & \multicolumn{1}{l|}{knife-peel-1}          & \multicolumn{1}{l|}{spheresmall-inspect-1}   & train-pass-1          \\ \hline
\multicolumn{1}{|l|}{bowl-pass-1}          & \multicolumn{1}{l|}{doorknob-use-2}           & \multicolumn{1}{l|}{lightbulb-pass-1}      & \multicolumn{1}{l|}{spheresmall-pass-1}      & train-play-1          \\ \hline
\multicolumn{1}{|l|}{camera-browse-1}      & \multicolumn{1}{l|}{duck-pass-1}              & \multicolumn{1}{l|}{lightbulb-screw-1}     & \multicolumn{1}{l|}{stamp-lift-1}            & watch-pass-1          \\ \hline
\multicolumn{1}{|l|}{camera-pass-1}        & \multicolumn{1}{l|}{elephant-inspect-1}       & \multicolumn{1}{l|}{mouse-lift-1}          & \multicolumn{1}{l|}{stamp-pass-1}            & waterbottle-drink-1   \\ \hline
\multicolumn{1}{|l|}{camera-takepicture-1} & \multicolumn{1}{l|}{elephant-pass-1}          & \multicolumn{1}{l|}{mouse-pass-1}          & \multicolumn{1}{l|}{stamp-stamp-1}           & waterbottle-pass-1    \\ \hline
\multicolumn{1}{|l|}{camera-takepicture-2} & \multicolumn{1}{l|}{eyeglasses-wear-1}        & \multicolumn{1}{l|}{mouse-use-1}           & \multicolumn{1}{l|}{stanfordbunny-inspect-1} & waterbottle-pour-1    \\ \hline
\multicolumn{1}{|l|}{camera-takepicture-3} & \multicolumn{1}{l|}{flashlight-on-1}          & \multicolumn{1}{l|}{mug-drink-1}           & \multicolumn{1}{l|}{stanfordbunny-lift-1}    & wineglass-drink-1     \\ \hline
\multicolumn{1}{|l|}{cubelarge-inspect-1}  & \multicolumn{1}{l|}{flashlight-on-2}          & \multicolumn{1}{l|}{mug-drink-2}           & \multicolumn{1}{l|}{stanfordbunny-pass-1}    & wineglass-drink-2     \\ \hline
\multicolumn{1}{|l|}{cubelarge-lift-1}     & \multicolumn{1}{l|}{flute-pass-1}             & \multicolumn{1}{l|}{mug-lift-1}            & \multicolumn{1}{l|}{stapler-lift-1}          & wineglass-lift-1      \\ \hline
\multicolumn{1}{|l|}{cubelarge-pass-1}     & \multicolumn{1}{l|}{flute-play-1}             & \multicolumn{1}{l|}{mug-pass-1}            & \multicolumn{1}{l|}{stapler-pass-1}          & wineglass-pass-1      \\ \hline
\multicolumn{1}{|l|}{cubemedium-inspect-1} & \multicolumn{1}{l|}{fryingpan-cook-1}         & \multicolumn{1}{l|}{mug-toast-1}           & \multicolumn{1}{l|}{stapler-staple-1}        & wineglass-toast-1     \\ \hline
\end{tabular}
}
\label{Table:subaction}
\end{table*}
