# Supplementary material for: QUAR-VLA: Vision-Language-Action Model for Quadruped Robots
Source: arXiv:2312.14457 source file (2025-02-04)
Supplement: Supplementary file 5 [file table_s_united.tex]

% SPGSN (AW)的结果和Wholebody的结果都需要更新，正在跑

% 30 没有A（w/o MMD loss; w/o DN）
% 31 # 没有A（w MMD loss; w/o DN）
% 32 没有A（w/0 MMD loss; w DN）
% 33  没有I（w/0 Phy; w/0 S）
% 34  没有I（w/0 Phy; w S）
% 35  没有I（w Phy; w/o S）

% 30 没有A,没有I（w/o MMD loss; w/o DN）
% 
%  \textbf{(3)} As to the key components of our method, we can observe that XCI is the most important design. With the help of XCA, the extracted interaction information is more expressive and lead to more high-fidelity prediction.

\begin{table}[h]
% \vspace{-1.5em}
\caption{{Average results on all actions with finer intervals.} }
\label{tab:s_wb}
\vspace{-.5em}
% 行距
\scriptsize
\centering
%cell大小
% \setlength{\aboverulesep}{1.85mm}
% \setlength{\belowrulesep}{-0.05mm}
\setlength{\tabcolsep}{0.72mm}{
\begin{tabular}{cc|cccccccccc}
\hline
 \multicolumn{2}{c|}{} &\multicolumn{10}{c}{Whole Body}\\
% \hline
\multicolumn{2}{c|}{Time (sec)}     & 0.1 & 0.2 & 0.3 & 0.4 & 0.5 & 0.6 & 0.7 & 0.8  & 0.9 & 1.0        \\
\hline
& LTD (D)~\cite{mao2019learning}

&7.5 &18.4 &30.9 &45.3&60.0 &73.9 &87.0 &100.3&112.4 &125.0\\
% & DMGNN (D)~\cite{li2020dynamic}  

% &23.0  &55.7  &107.7  &131.4
% \\
% &{PGBIG (D)~\cite{ma2022progressively}} 

% &22.6  &53.6  &104.3  &129.6
% \\
% 右手的结果需要更新
\multirow{-4}{*}{\rotatebox[origin=c]{90}{\cellcolor{white}\textbf{}}}
& {SPGSN (D)~\cite{li2022skeleton}}

&8.7 &21.2 &34.9 &48.4&62.0 &75.3 &87.9 &100.3&112.4 &124.0\\

\hline
\hline
% RH 结果有点问题，需要重新训练
{\cellcolor{white}} & {\cellcolor{white}LTD (U)~\cite{mao2019learning}}

&7.4 &18.4 &30.5 &43.1&55.9 &68.5 &81.6 &95.2&108.2 &120.4\\
% &Res. sup.~\cite{martinez2017human}& \\
% {\cellcolor{white}} & DMGNN (U)~\cite{li2020dynamic}  

% &22.7  &50.0 &98.9  &128.2
% \\
% {\cellcolor{white}} &{PGBIG (U)~\cite{ma2022progressively}} 

% &22.2  &48.1  &97.4  &125.8
% \\
{\cellcolor{white}} & {SPGSN (U)~\cite{li2022skeleton}}   

&8.9 &21.0 &34.3 &46.9 &60.3 &72.6 &84.5 &96.3 &107.7 &120.3

\\
\hline
\hline

\multirow{-7}{*}{\rotatebox[origin=c]{90}{\cellcolor{white}\textbf{}}}

& {\cellcolor{white}\textbf{EAI} (Ours)}

&\textbf{6.4} &\textbf{16.7} &\textbf{28.6} &\textbf{40.7}&\textbf{52.5} &\textbf{63.7} &\textbf{75.0} &\textbf{85.8}&\textbf{95.2} &\textbf{104.6}
\\
\bottomrule

\end{tabular}
}
\vspace{-.5em}
\end{table}
