# Supplementary material for: QUAR-VLA: Vision-Language-Action Model for Quadruped Robots
Source: arXiv:2312.14457 source file (2025-02-04)
Supplement: Supplementary file 6 [file first_section.tex]

\vspace{-1.5cm}
\begin{center}
\begin{large}
  \textbf{Abstract}
\vspace{-.2cm}  
\end{large}
\end{center}
\vspace{-.2cm}
\small
This supplementary material provides more information and additional experiments that could not be included in the main article due to space limitations. The document is organized as:
\vspace{-.1cm}
\begin{itemize}
\item[$\bullet$] In (\textbf{Sec: 1. Details of QUART}), we show more details of the data model structure and training strategy. 
\end{itemize}
\vspace{-.4cm}

\begin{itemize}
\item[$\bullet$] In (\textbf{Sec: 3. More results}), we provide additional results of the .
\end{itemize}

%%%%%%%%%%%%%%%%%%%
