# Supplementary material for: QUAR-VLA: Vision-Language-Action Model for Quadruped Robots
Source: arXiv:2312.14457 source file (2025-02-04)
Supplement: Supplementary file 7 [file table_s_ab1.tex]

% 需要添加更多的指标,比如说拿出几个类别作为例子，剩下类别的结果放在补充材料上

% 60 Intra-encoder: 9
% 61 Intra-encoder: 6
% 62 Intra-encoder: 3
% 63 Intra-encoder: 15
% 64 ca_layer:2
% 65 ca_layer:3
% 66 ca_layer:4
% 67 ca_layer:6
% 68 predictor mlp:2
% 69 predictor mlp:3
% 70 predictor gcn
% 71 intra-encoder: st-transformer

\begin{table}[!ht]
\scriptsize
% 行距
\centering
\caption{{Ablation experiments on the GCN numbers of intra-context encoder.} 
}
\vspace{-1em}
\resizebox{1\linewidth}{!}{
\begin{tabular}{c|ccccc|cccc}
\hline
 {Num of GCN} &{3}&{6} & {9} & {12} & {15}    &0.2s  & 0.4s  & 0.8s  & 1.0s   
\\ 
\hline
\cellcolor{white} &{\checkmark} &  & & &   &{16.5} &{42.1} &93.4 &113.7    
\\
\cellcolor{white}& &\checkmark  &  &&   &{16.4} &41.5 &{92.7} &{112.5}  
\\
\cellcolor{white}& &  &\checkmark  & &  &\textbf{16.3} &\textbf{40.4} &{89.2} &{109.4}  
\\
\multirow{-3}{*}{{\cellcolor{white}\textbf{Variants}}}
{\cellcolor{white}} 
& &  & & & \checkmark  &{16.2} &40.7 &89.1 &107.6 \\ 
            
\hline
{\textbf{EAI}}& &  &  & \checkmark &  & {16.7} & {40.7} & \textbf{85.8} & \textbf{104.6}  \\
\bottomrule
\end{tabular}
}
\vspace{-0.25cm}
\label{tab:s_ab_gcnnum}
\end{table}
