# Supplementary material for: QUAR-VLA: Vision-Language-Action Model for Quadruped Robots
Source: arXiv:2312.14457 source file (2025-02-04)
Supplement: Supplementary file 9 [file table_s_ab3.tex]

% 需要添加更多的指标,比如说拿出几个类别作为例子，剩下类别的结果放在补充材料上

% 60 Intra-encoder: 9
% 61 Intra-encoder: 6
% 62 Intra-encoder: 3
% 63 Intra-encoder: 15
% 64 ca_layer:2
% 65 ca_layer:3
% 66 ca_layer:4
% 67 ca_layer:6
% 68 predictor mlp:2
% 69 predictor mlp:3
% 70 predictor gcn
% 71 intra-encoder: st-transformer
\vspace{-.2cm}
\begin{table}[!ht]
\scriptsize
% 行距
\centering
\caption{{Ablation experiments of predictor.} 
}
% \vspace{-1em}
\resizebox{1\linewidth}{!}{
\begin{tabular}{c|cccc|cccc}
\hline
 {} &{1-MLP} &{2-MLPs}&{3-MLPs} & {GCN}   &0.2s  & 0.4s  & 0.8s  & 1.0s 
\\ 
\hline
\cellcolor{white} & & {\checkmark} & &   &{17.0} &{40.9} &86.5 &107.6 
\\
\cellcolor{white}& &  & {\checkmark} &   &{17.8} &\textbf{40.3} &{86.3} &{107.0}  
\\
\multirow{-3}{*}{{\cellcolor{white}\textbf{Variants}}}
\cellcolor{white}& &  &  &{\checkmark}   &\textbf{16.6} &41.9 &{92.6} &{114.4} 
\\

\hline
{\textbf{EAI}}&\checkmark &   &  &  & {16.7} & {40.7} & \textbf{85.8} & \textbf{104.6}  \\
\bottomrule
\end{tabular}
}
% \vspace{-0.1cm}
\label{tab:s_ab_pred}
\end{table}
