# Supplementary material for: QUAR-VLA: Vision-Language-Action Model for Quadruped Robots
Source: arXiv:2312.14457 source file (2025-02-04)
Supplement: Supplementary file 10 [file table_s_ab4.tex]

% 需要添加更多的指标,比如说拿出几个类别作为例子，剩下类别的结果放在补充材料上

% 60 Intra-encoder: 9
% 61 Intra-encoder: 6
% 62 Intra-encoder: 3
% 63 Intra-encoder: 15
% 64 ca_layer:2
% 65 ca_layer:3
% 66 ca_layer:4
% 67 ca_layer:6
% 68 predictor mlp:2
% 69 predictor mlp:3
% 70 predictor gcn
% 71 intra-encoder: st-transformer

\vspace{-.2cm}
\begin{table}[!ht]
\scriptsize
% 行距
\centering
\caption{{Ablation experiments of intra-context encoder types.} 
}
\vspace{-1em}
\resizebox{1\linewidth}{!}{
\begin{tabular}{c|cc|cccc}
\hline
 {Type of Intra-encoder} &{GCN}&{ST-Transformer}    &0.2s  & 0.4s  & 0.8s  & 1.0s   
\\ 
\hline
\multirow{-1}{*}{{\cellcolor{white}\textbf{Variants}}}
\cellcolor{white} & & {\checkmark}   &{17.4} &{43.7} &90.4 &109.8 
\\
            
\hline
{\textbf{EAI}} & \checkmark &  & \textbf{16.7} & \textbf{40.7} & \textbf{85.8} & \textbf{104.6} \\
\bottomrule
\end{tabular}
}
\vspace{-0.25cm}
\label{tab:s_ab_intra}
\end{table}
