# Supplementary material for: QUAR-VLA: Vision-Language-Action Model for Quadruped Robots
Source: arXiv:2312.14457 source file (2025-02-04)
Supplement: Supplementary file 11 [file table_s_ab_g.tex]

\begin{table}[htb]
\vspace{-.em}
\caption{{Generalization experiment on AMASS.} }
\label{tab:r_amass}
\vspace{-.8em}
% 行距
\footnotesize
\centering
\setlength{\tabcolsep}{3mm}{
\begin{tabular}{cc|cccc}
% \multicolumn{2}{c|}{} &\multicolumn{4}{c}{whole-body} \\
\hline
\multicolumn{2}{c|}{Time (sec)}     & 0.2 & 0.4  & 0.8  & 1.0\\  
\hline
 & {LTD (U)}	
&21.5  &55.8  &86.1 &117.5 \\
& {SPGSN (U)} 
&21.8 &55.3 &79.7  &110.8 \\

\hline
& {\textbf{EAI} (Ours)}
						 		
&\textbf{19.5  } &\textbf{55.0}&\textbf{76.5} &\textbf{102.6 }\\
\bottomrule
\end{tabular}
}
\vspace{-.5em}
\end{table}
